# Supplementary material for: Individual Fairness in Graph Decomposition
Source: arXiv:2406.00213 source file (2024-05-31)
Supplement: Supplementary file 1 [file figures_appendix.tex]

\section{Additional Figures}

\begin{figure}[htbp]
\centering
\includegraphics[width=0.5\linewidth]{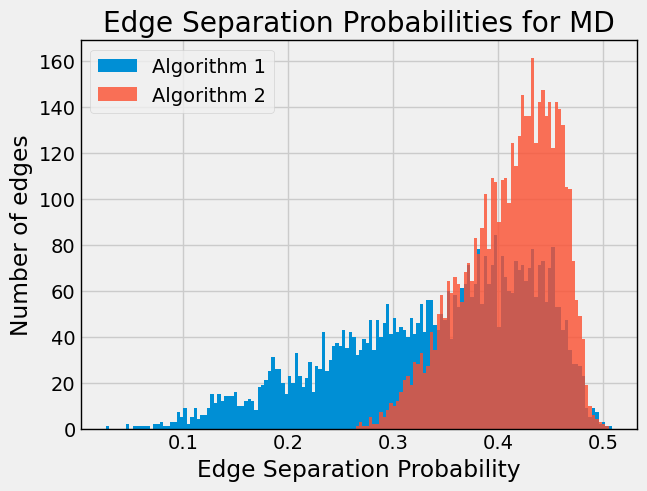}
\caption{Histogram of edge separation probabilities across 3000 runs of \cref{alg:kpr-randwts} on Maryland.
\label{fig:gaussianMD}
}
\end{figure}

\begin{figure}[htbp]
\centering
\includegraphics[width=0.5\linewidth]{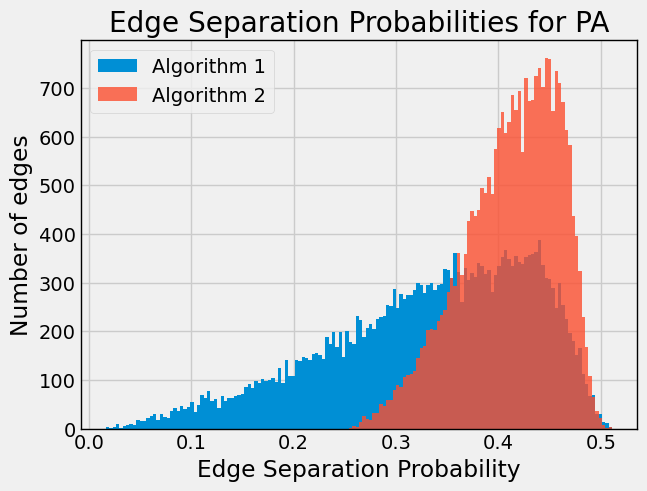}
\caption{Histogram of edge separation probabilities across 3000 runs of \cref{alg:kpr-randwts} on Pennsylvania.
\label{fig:gaussianPA}
}
\end{figure}
